# Supplementary material for: LCNN: Lookup-based Convolutional Neural Network
Source: arXiv:1611.06473 source file (2017-06-13)
Supplement: Supplementary file 1 [file supp-mat.tex]

\begin{figure*}[!thb]
    \centering
    \small
    \begin{tabular}{|l | c | c | c | c | c | c | c | c | c |}
     \hline
     \textbf{AlexNet} & conv1 & conv2 & conv3 & conv4 & conv5 & fc6 & fc7 & fc8 & overall\\
     \hline
     computation \% & $9.29\%$ & $39.45\%$ & $13.17\%$ & $19.76\%$ & $13.17\%$ & $3.33\%$ & $1.48\%$ & $0.36\%$ & $100\%$\\
     \Xhline{4\arrayrulewidth}
     Wen \etal~\cite{wen2016learning} & $1.05\times$ & $3.37\times$ & $6.27\times$ & $9.73\times$ & $4.93\times$ & $1\times$ & $1\times$ & $1\times$ & $3.1\times$\\
     \hline
     XNOR-Net~\cite{Rastegari2016XNORNetIC} & $1\times$ & $32\times$ & $32\times$ & $32\times$ & $32\times$ & $32\times$ & $32\times$ & $1\times$ & $8.0\times$\\
     \hline
     LCNN-fast & $16.66\times$ & $80.24\times$ & $83.23\times$ & $75.47\times$ & $61.99\times$ & $7.73\times$ & $7.91\times$ & $1\times$ & $37.6\times$\\
     \hline
     LCNN-accurate & $6.97\times$ & $2.57\times$ & $3.51\times$ & $3.75\times$ & $3.21\times$ & $3.14\times$ & $3.83\times$ & $1\times$ & $3.2\times$\\
     \hline
    \end{tabular}
    \caption{\small Comparing the layer-wise speedup of each model on AlexNet. The accuracy of each model is reported in the paper.}
    \label{tab:alexnetlayers}
\end{figure*}

\section{Layer-wise speedup}

In this section we compare the layer-wise speedup of LCNN with the baselines. In AlexNet most of the computation is done in the early layers, where the input size is still large. Table~\ref{tab:alexnetlayers} shows the percentage of the computation in each layer of AlexNet and the speedup gain of each model on each layer. XNOR-Net~\cite{Rastegari2016XNORNetIC} gets $32\times$ speedup on $32$-bit machines, and it is higher for $64$-bit or $128$-bit machines. However, since they don't binarize the first layer, and $9.29\%$ of computation is done in the first layer, their speedup is bound by $\frac{1}{9.29\%}=10.8\times$ speedup. This is still much lower than LCNN-fast speedup, which gets about the same accuracy. Wen \etal~\cite{wen2016learning} gets good speedup on conv2-5, yet their speedup is much lower on the first layer. We think this is because they're sparsifying the weight tensors themselves. The weight tensor in the first layer cannot be very sparse as their goal is extract low lever features. LCNN-accurate, however, is speeding up the first layer by representing the weight tensor by a sparse combination of a set of vectors.

\begin{figure*}
\centering
\subfigure[Trial \#1 categories:\\
    \begin{tabular}{lcl}
        1-  & \texttt{n01514859} & hen.n.02 \\
        2-  & \texttt{n01773549} & barn\_spider.n.01 \\
        3-  & \texttt{n01978287} & dungeness\_crab.n.02 \\
        4-  & \texttt{n02099429} & curly-coated\_retriever.n.01 \\
        5-  & \texttt{n02669723} & academic\_gown.n.01 \\
        6-  & \texttt{n03888257} & parachute.n.01 \\
        7-  & \texttt{n03995372} & power\_drill.n.01 \\
        8-  & \texttt{n04005630} & prison.n.01 \\
        9-  & \texttt{n04467665} & trailer\_truck.n.01 \\
        10-  & \texttt{n13133613} & ear.n.05 \\
    \end{tabular}]{
  \includegraphics[width=0.25\textwidth]{sections/figs/fewexample-random5}
%   \label{fig:randomfew}
}
\hspace{20mm}
\subfigure[Trial \#2 categories:\\
    \begin{tabular}{lcl}
        1-   & \texttt{n01983481} & american\_lobster.n.02 \\
        2-   & \texttt{n02091467} & norwegian\_elkhound.n.01 \\
        3-   & \texttt{n02444819} & otter.n.02 \\
        4-   & \texttt{n02607072} & anemone\_fish.n.01 \\
        5-   & \texttt{n02817516} & bearskin.n.02 \\
        6-   & \texttt{n02879718} & bow.n.04 \\
        7-   & \texttt{n03530642} & honeycomb.n.02 \\
        8-   & \texttt{n03908618} & pencil\_box.n.01 \\
        9-   & \texttt{n04286575} & spotlight.n.02 \\
        10-  & \texttt{n04554684} & washer.n.03 \\
    \end{tabular}]{
  \includegraphics[width=0.25\textwidth]{sections/figs/fewexample-random4}
%   \label{fig:randomfew}
}
\hfill
\subfigure[Trial \#3 categories:\\
    \begin{tabular}{lcl}
        1-  & \texttt{n02110063} & malamute.n.01\\
        2-  & \texttt{n02111277} & newfoundland.n.01\\
        3-  & \texttt{n03724870} & mask.n.01\\
        4-  & \texttt{n03775546} & mixing\_bowl.n.01\\
        5-  & \texttt{n03782006} & monitor.n.05\\
        6-  & \texttt{n03929660} & pick.n.05\\
        7-  & \texttt{n04201297} & shoji.n.01\\
        8-  & \texttt{n04487081} & trolleybus.n.01\\
        9-  & \texttt{n07753113} & fig.n.04\\
        10- & \texttt{n07930864} & cup.n.06\\
    \end{tabular}]{
  \includegraphics[width=0.25\textwidth]{sections/figs/fewexample-random3}
%   \label{fig:randomfew}
}
\vspace{20mm}
\subfigure[Trial \#4 categories:\\
    \begin{tabular}{lcl}
        1-  & \texttt{n01669191}    & box\_turtle.n.01 \\
        2-  & \texttt{n01773157}    & black\_and\_gold\_garden\_spider.n.01 \\
        3-  & \texttt{n02106662}    & german\_shepherd.n.01 \\
        4-  & \texttt{n03733131}    & maypole.n.01 \\
        5-  & \texttt{n03929855}    & pickelhaube.n.01 \\
        6-  & \texttt{n04116512}    & rubber\_eraser.n.01 \\
        7-  & \texttt{n04389033}    & tank.n.01 \\
        8-  & \texttt{n04590129}    & window\_shade.n.01 \\
        9-  & \texttt{n04592741}    & wing.n.02 \\
        10- & \texttt{n07836838}    & chocolate\_sauce.n.01 \\
    \end{tabular}
    ]
{
  \includegraphics[width=0.25\textwidth]{sections/figs/fewexample-random1}
%   \label{fig:nocatsofabike}
}
\hfill
\subfigure[Trial \#5 categories:\\
    \begin{tabular}{lcl}
        1-  & \texttt{n01774384} & black\_widow.n.01\\
        2-  & \texttt{n02090379} & redbone.n.01\\
        3-  & \texttt{n02113023} & pembroke.n.01\\
        4-  & \texttt{n02138441} & meerkat.n.01\\
        5-  & \texttt{n02444819} & otter.n.02\\
        6-  & \texttt{n02917067} & bullet\_train.n.01\\
        7-  & \texttt{n03016953} & chiffonier.n.01\\
        8-  & \texttt{n03180011} & desktop\_computer.n.01\\
        9-  & \texttt{n03207941} & dishwasher.n.01\\
        10- & \texttt{n03476684} & hair\_slide.n.01\\
    \end{tabular}]{
  \includegraphics[width=0.25\textwidth]{sections/figs/fewexample-random2}
%   \label{fig:randomfew}
}
\vspace{-2cm}
\caption{\small Comparing LCNN and standard CNN on few-example training. LCNN beats standard CNN in all samplings.}
\label{fig:fewexample}
\end{figure*}

\section{Few-example trials}
We do the few-example experiment under two settings: \begin{inparaenum}\item Try $5$ random samplings of $10$ random categories for few-example training and report the average over all. \item Set aside all cats ($7$ categories), bicycles ($2$ categories) and sofa ($1$ category)\end{inparaenum}. Here we report exactly which categories have been excluded in each trial and the accuracy of LCNN and CNN on each trial. At each trial we try $10$ random samplings of few examples from the training set of ILSVRC2012. Figure \ref{fig:fewexample}
